# Supplementary material for: DReAM: Dynamic Re-arrangement of Address Mapping to Improve the Performance of DRAMs
Source: arXiv:1509.03721 source file (2015-09-12)
Supplement: Supplementary file 1 [file Appendix.tex]

\newpage
\section{Appendix}
\label{sec:appendix}

%===== Migration Scenarios ====

\subsubsection{Scenario 2 - Online Data Migration using Non-Volatile Memory Technology} \label{subsubsec:dream_scenario_2}

This scenario takes advantage of a novel non-volatile DIMM structure, that includes flash devices in the same DIMM as DRAM, to avoid rebooting the system required by the first scenario. For instance, ArxCis-NV \cite{website:vikingTech1,website:vikingTech2,sartakovnv} is a non-volatile DDR3 DIMM which is already available in the market, produced by Viking Technology \cite{website:vikingTech3}. The preliminary aim of ArxCis-NV is to preserve critical data in the event of power or system failure. This memory structure continuously monitors voltage levels from the host system and, in the case of voltage drop, triggers a SAVE function which mirrors DRAM states to the flash memory. In this situation, ArxCis-NV uses backup power provided by embedded supercapacitors to transfer data into the non-volatile flash. At the reboot time data will be restored from flash similarly. 

DReAM will use the functionality provided by ArxCis-NV in a slightly different manner. The only difference is that the ArxCis-NV triggers the SAVE functions in the case of voltage drop but DReAM would trigger the SAVE function whenever a new address-mapping scheme is detected at application run-time. Therefore, the existing data in the DRAM will read using the pre-defined address-mapping scheme and copy to the flash, and after that, data will be restored to the DRAM using the predicted address-mapping scheme. According to the datasheet of ArxCis-NV  the read and write bandwidth of this module is 4~GB/s which means the content of 4~GB DRAM can be copied in 1 second and restored in 1 second \cite{website:vikingTech4}. Therefore, there is 2 seconds penalty each time that DReAM changes the address mapping scheme. This delay is much smaller than the delay imposed by rebooting the system. 

\subsubsection{Scenario 3 - Online Data Migration using NanoCommit} \label{subsubsec:dream_scenario_3}

Although, the second scenario imposes a lower overhead for the data migration process than the first scenario in reality there is no need to copy all the data back from flash when the address-mapping is changed. The reason is that some of the existing data in DRAM might not be needed anymore by the application. Thus, a more elegant approach would be to return data to the memory only when it has been requested again. To demonstrate this scenario, Memory Channel Storage (MSC)~\cite{website:diabloTech2} and NanoCommit technology \cite{website:diabloTech3} can be used which are invented by Diablo Technology \cite{website:diabloTech1}.

The main principles behind MSC is to bypass the traditional interface between non-volatile memory (e.g. flash) and memory subsystem to provide a shorter and faster path from a CPU to the massive data storage offered by non-volatile memories. Similar, to the second scenario, MSC also employs flash memory on the same DIMM that houses DRAMs. Diablo Technology has invented another technology on top of MSC which is called NanoCommit \cite{website:diabloTech3}. Using NanoCommit, all the write operation to the DRAM devices will be also written to the flash memory with a latency of 48~ns. This allows that DRAM modifications to be rapidly made persistent in flash.

DReAM can take advantage of MSC and NanoCommit to mitigate the cost of online data migration. Assuming that MSC and NanoCommit are in place, in the case of any changes in address-mapping scheme using DReAM, there is no need to copy DRAM contents to the flash since data is already in flash. On the other hand, as discussed, there is no need to copy all the data back to DRAMs from flash before any access to data. A more efficient solution is to move data from flash to the DRAMs based on the memory requests. Therefore, there is no unnecessary cost for migrating data which are not needed anymore. This reduce the cost of data migration significantly in comparison with scenario~2.

%===== Bulk Data Copy ====
\begin{itemize}

\item {\bf Intra-subarray:} In this scenario, source and destination rows share the same row-buffer. Therefore, the copying process involves two main steps: (1) loading the source row into the row-buffer and (2) loading the row-buffer into the destination row. The first step can be easily done by activating the source row which connects the bitlines of the source row to the row-buffer. Therefore, the source row will be loaded into the row-buffer. The next step is simply copy the row-buffer contents to the destination row by connecting the bitlines of the destination row to the row-buffer. However, it is not possible since the source row is still connected to the row-buffer (its wordline is raised) and the original implementation of DRAMs do not allow raising two wordlines at the same time. This is because all the rows within the same bank share one row-decoder. On the other hand, although precharging the source row lowers the wordline of the source row it also clear the row-buffer contents. To solve this issue, Seshadri \textit{et al}.\ \cite{seshadri2013rowclone} proposed a new DRAM command called DEACTIVATION that only lowers the wordline of the source row without clearing the row-buffer. Therefore, after issuing the DEACTIVATION command to the source row, the destination row can be activated using an Activation command. Hence, the content of row-buffer will be loaded to the destination row. As they evaluated, this scenario requires the minimal modification to DRAM device, 0.0016\% die-size overhead.

\item {\bf Inter-subarray:} In this scenario, source and destination rows located in different subarrays. Therefore, it is not possible to use the wide bitline/row-buffer communication bus to transfer data. Instead, data must be transferred using the 64-bit I/O bus that connects to all the row-buffers inside the same bank as well as to all the row-buffers in different banks. Intuitively, since both subarrays are in the same bank, it is possible to read from source row-buffer from one subarray and write to the destination row-buffer in different subarray. However, the first problem is that the the original read or write commands transfer data on the I/O bus to/from the DRAM device's data-pins which is unnecessary for the purpose of copying data inside DRAM. Therefore, Seshadri \textit{et al}.\ \cite{seshadri2013rowclone} proposed a new DRAM command called TRANSFER that reads data from source row-buffer and writes it to the destination row-buffer using I/O bus without transferring data to the chip's data pins. To copy the entire row multiple TRANSFER commands must be issued by the memory controller. Seshadri \textit{et al}. investigated that the additional control logic to implement the TRANSFER command (disconnect the I/O bus from data pins) incurs a negligible 0.01\% die size increase \cite{seshadri2013rowclone}. 

On the other hand, since both subarrays use the same bank's I/O buffer to perform the read and write operation then the bank's I/O buffer has to switch between reading data from the source row-buffer (64-bit) and writing data to the destination row-buffer (64-bit). As discussed in Chapter~\ref{cha:background}, there is a cost associated with I/O switching between read and write operation. To work around this issue, Seshadri \textit{et al}.\ \cite{seshadri2013rowclone} proposed saving one row in each bank as a temporary buffer to first copy data from source row-buffer to a different bank and then to write it back to the destination row buffer. In this way the source bank's I/O buffer only performs the read and the destination bank's I/O only performs the write operation. They state that the capacity loss associated with one temporary buffer per bank is negligible, 0.0015\%.

\item {\bf Intra-bank:} this scenario is similar to the previous scenario with one difference; since the source and destination rows are in different banks then they do not share a row-decoder. Therefore, both source and destination rows can be activated at the same time in different banks. Thus, the content of source row-buffer can be transferred using several TRANSFER commands to the destination row-buffer.   

\end{itemize}

%==== inter subarray and intra subarray migration
{\bf Intra-subarray Migration:} In this scenario (\ref{fig:intra_subarray_mig}), source and destination rows are both in the same subarray. Therefore to perform the migration and swap operation the following procedure will be followed.
\begin{enumerate}
\item Activate the source row and load its contents into the global row-buffer.
\item	Activate the destination row locally and load its contents to the local row-buffer~1. 
\item Connect the local bitline of source row to the local row-buffer. This will copy the destination row to the source row.
\item Connect the global row-buffer to the destination row. This will copy the source row to the destination row.
\end{enumerate}

{\bf Inter-subarray Migration:} In this scenario (\ref{fig:inter_subarray_mig}), source and destination rows are in different subarrays within the same bank. One possible way to swap data in source and destination is to make a copy of source row in the global row-buffer and then use the narrow I/O bus to transfer the destination row from the local row-buffer 2 to the local row-buffer one. Finally copy the source row from the global row buffer to the local row-buffer two and then to the destination row. However, there is only one I/O per bank which will be used for read and write operation. As discussed before, reading from one row-buffer and writing back to the another row-buffer imposes extra penalty each time the I/O switches between read and write mode. To workaround this issue, the following procedure is suggested to perform the migration and swap process in this scenario.
\begin{enumerate}
\item Activate the source row to the global row-buffer and destination row to the local row-buffer 2.
\item Transfer the source row (located in the global row buffer of bank A) to the global row-buffer of bank B using the narrow I/O bus.
\item Connect the global bitlines of bank A to the local row-buffer 2 to load its content the global row buffer.
\item Connect the global row-buffer of bank A to the local row-buffer 1 and the source row. This will copy the destination row to the source row.
\item Transfer source row from the global row-buffer in bank B to the local row-buffer 2 in bank A.
\item Connect the local bitlines of the local row-buffer 2 to the destination row. This will copy the source row to the destination row.
\end{enumerate}

% Inter vs Intra bank migration
\begin{figure}[!htb]
\centering
\includegraphics[scale=0.1]{Figures/Data_Relocation}
\caption{The analysis of inter and intra bank data relocation required by DReAM online.}
\label{fig:data_relocation}
\end{figure}

% memory footprint
\begin{figure}[!htb]
\centering
\includegraphics[scale=0.15]{Figures/DReAM_Partial_Migration_Cost}
\caption{Associated cost of partial data migration for DReAM.}
\label{fig:partial_migration_cost}
\end{figure}

%==== Detailed motivative results

\begin{figure*}

\centering
\includegraphics[scale=0.29]{Figures/Motivation_Address_Mapping}
\caption{Performance comparison amongst different\\ address-mapping schemes.}
\label{fig:motivation_address_mapping}

\centering
\includegraphics[scale=0.25]{Figures/Mapping_Result_Commercial}
\caption{Address mapping profiling for BIOBENCH and COMMERCIAL benchmark suites.}
\label{fig:comparision_comercial}

\centering
\includegraphics[scale=0.25]{Figures/Mapping_Result_HPC}
\caption{Address mapping profiling for HPC benchmarks.}
\label{fig:comparision_hpc}

\centering
\includegraphics[scale=0.25]{Figures/Mapping_Result_PARSEC}
\caption{Address mapping profiling for PARSEC benchmark suite.}
\label{fig:comparision_parsec}

\centering
\includegraphics[scale=0.25]{Figures/Mapping_Result_SPEC}
\caption{Address mapping profiling for SPEC benchmark suite.}
\label{fig:comparision_spec}

\end{figure*}
